# Supplementary material for: A Category Theoretic View of Contextual Types: from Simple Types to Dependent Types
Source: arXiv:2206.02831 source file (2022-06-08)
Supplement: Supplementary file 1 [file appendix.tex]

\clearpage

\section{Structure of the Presheaf Category}

In the main text, we have explained the structure of~$\hat\CC$ in terms of
its internal dependent type theory.
Here we explain in more detail how the internal dependent type theory
relates to the direct definition of $\hat\CC$ as a functor category.

\subsection{Basic Structure}

To fix notation, we recall the basic structure of $\hat\CC$.

\subsubsection{Finite Limits and Colimits}

Finite limits and colimits exist and are constructed pointwise.
In particular, finite products and coproducts are given by:
\begin{align*}
  1(\Gamma) &= \{*\}
  &
    (X\times Y)(\Gamma)
  &= X(\Gamma)\times Y(\Gamma)
  \\
  0(\Gamma) &= \emptyset
  &
    (X + Y)(\Gamma)
  &= X(\Gamma) + Y(\Gamma)
\end{align*}
The Yoneda embedding preserves finite products.

\subsubsection{Exponentials}

The category $\hat\CC$ has exponentials.
The exponential $(X\Rightarrow Y)$ can be calculated using the Yoneda lemma.
We recall that the Yoneda lemma states that $Z(\Gamma)$ is naturally
isomorphic to $\hat\CC(\y(\Gamma), Z)$.
With this, we have:
\[
  (X\Rightarrow Y)(\Gamma)
  \ \iso\ \hat\CC(\y(\Gamma), X \Rightarrow Y)
  \ \iso\ \hat\CC(\y(\Gamma) \times X , Y)
\]
Since~$\y$ preserves finite products, we have in particular
$(\y(A) \Rightarrow \y(B))(\Gamma)
\iso \hat\CC(\y(\Gamma) \times \y(A) , \y(B))
\iso \hat\CC(\y(\Gamma \times A) , \y(B))
\iso \CC(\Gamma \times A, B)$.
In the case where $A=B=\tm$, this shows that the exponential $\tm \Rightarrow \tm$
represents terms with an additional bound variable.

\subsubsection{Subobject Classifier}

The category $\hat\CC$ has a subobject classifier.
This is a map $\top \colon 1 \to \Omega$ such that, for any
monomorphism~$m$ there is a unique map $\xi$ making
the diagram below a pullback.
\begin{equation*}
  \xymatrix{
    Y\ar[r] \ar@{ >->}[d]_{m}
    \pullbackcorner[ul]
    & 1\ar[d]^\top
    \\
    X\ar@{-->}[r]_{\chi} & \Omega
  }
\end{equation*}
When given $\chi\colon X \to \Omega$, one can obtain the a morphism $m_\chi\colon \{\chi\} \mono X$ by
pullback of $\top$ along $\chi$, as in the diagram.
We can choose this morphism such that, at any stage~$\Gamma$, it is just subset inclusion.
This means that $\{\chi\}(\Gamma) \subseteq X(\Gamma)$ holds for all $\Gamma$ and that
$\left(m_\chi\right)_\Gamma$ is the inclusion function.
%
%TODO: Subobjects are point-wise subsets

\subsubsection{Partial Maps}

As any elementary topos, $\hat\CC$ has a partial map classifier.
It may be constructed as follows.
Given~$Y$ in~$\hat\CC$, let $Y_\bot$ be the presheaf obtained from $Y$ by
disjointly adding an element~$\bot$ to each~$Y(\Gamma)$.
We assume that this is done such that $Y(\Gamma)\subseteq Y_\bot(\Gamma)$ holds.
We then define $X \parmap Y$ as $X \Rightarrow Y_\bot$.
This object represents partial maps from~$X$ to~$Y$.

\subsection{Dependent Types in a Presheaf Category}
% TODO: If we're using CwAs later, then maybe it's best to use them here too

Presheaf categories have enough structure to model dependent types.
One can think of the interpretation of dependent types as a slight generalisation of the
set-theoretic interpretation of dependent types, where a type $\Phi \vdash X \type$ is
interpreted by a base set~$B$ and a predicate~$\phi$.
With this data, the dependent type amounts to the set
$\{(p, x) \mid p\in \Phi, x\in B, \phi(p, x)\}$.
This standard construction works in the internal set-theory of any topos and so in
particular in presheaf categories.

To interpret a dependent type theory in~$\hat\CC$, it suffices to show
that $\hat\CC$ has the structure of a CwA and to
use an existing interpretation of the syntax, e.g.~\cite{Hofmann:NI97}, in this structure.

A Category with Attributes for~$\hat\CC$ is defined as follows.
\begin{itemize}
\item The category of contexts $\mathrm{Ctx}$ is $\hat \CC$ itself.

\item
  The functor $\mathrm{Ty} \colon \op{\mathrm{Ctx}} \to \mathrm{Set}$ is defined as follows.

  The set $\mathrm{Ty}(\Phi)$ is defined to be the set of all pairs $X = (B, \chi)$
  where~$B$ is an object of~$\hat \CC$ and $\phi \colon \Phi \times B \to \Omega$ is a
  predicate on~$\Phi \times B$.
  The intuition is that this defines a dependent type $p\colon \Phi \vdash X(\phi)$ by
  $X(\phi) = \{ x \in B \mid \chi(\phi, x) = \top \}$.  Thus, the object~$B$ is a
  non-dependent type that can uniformly encode the values of the dependent type for
  arbitrary dependency, and $\phi$ formalises which dependencies are possible.

  Type substitution is defined by pre-composition. If $\sigma\colon \Psi \to \Phi$ is a
  morphism in $\mathrm{Ctx}$ and $X=(B, \chi)$ is a type, then $\mathrm{Ty}(\sigma)(X)$ is
  defined to be $(B, \chi \circ (\sigma \times B))$.
  We write $\sigma^*X$ for $\mathrm{Ty}(\sigma)(X)$.

\item For each type $X\in \mathrm{Ty}(\Phi)$, there must be an object $\Phi \ltimes X$ in
  $\mathrm{Ctx}$ and a projection morphism $\pi_X \colon \Phi \ltimes X \to \Phi$.

  In the case of~$\hat\CC$, the predicate
  $\chi \colon \Phi \times B \to \Omega$ in the type $X=(B,\chi)$
  induces a monomorphism  $m_\chi \colon \{\chi\} \mono \Phi \times B$.
  We define $(\Phi \ltimes X)$ to be its domain $\{\chi\}$.
  The notation symbolises the intuition that $(\Phi \ltimes X)$ consists
  of all pairs $(p, x)$ with $p\colon \Phi$ and $x\colon X(p)$.
  The projection morphism $\pi_X\colon (\Phi \ltimes X) \to \Phi$ is defined by
  $\pi_X := \pi_1\circ m_\chi$.

\item
  Finally, for each $\sigma \colon \Psi \to \Phi$ and each $X\in \mathrm{Ty}(\Phi)$,
  there must be a morphism
  $q(\sigma,X) \colon \Psi \ltimes \mathrm{Ty}(\sigma)(X) \to \Phi \ltimes X$
  making the following diagram a pullback.
  \[
    \xymatrix@C=2cm{
      \Psi \ltimes \mathrm{Ty}(\sigma)(X)
      \ar[r]^-{q(\sigma, X)}
      \ar[d]_{\pi}
      \pullbackcorner[ul]
      &
       \Phi \ltimes X
      \ar[d]^{\pi}
      \\
      \Psi
      \ar[r]_{\sigma}
      &
      \Phi
    }
  \]

  In the case of $\hat\CC$, notice that  $\Phi \ltimes X$ and $\Psi \ltimes \mathrm{Ty}(\sigma)(X)$
  are subobjects of $\Phi \times B$ and $\Psi \times B$ for the same~$B$.
  The map $q(\sigma,X)$ is the unique morphism over $\sigma \times B$. % TODO: haven't said what 'over' means
\end{itemize}

This interpretation of dependent types is equivalent to approaches using display maps
or the codomain fibration~\cite{Jacobs:TCS93}.
In these approaches, types are simply given by their projection maps~$\pi_X$.
The advantage of the above representation of $\pi_X$ as a pair $(B,\chi)$ is that it comes
with a suitable choice of the objects~$\sigma^*X$, which are otherwise only determined up
to isomorphism by pullbacks.
This is important for the interpretation of syntax, as in~\cite{streicher91}.
The construction amounts to a splitting of the codomain fibration for~$\hat\CC$.

\subsection{Type Formers}

To outline the interpretation of the type theoretic presentation of the structure of $\hat\CC$ from
the main text, we need to spell out concretely the interpretation of the type formers for products
and identity types.

To this end, notice that to define a type $X=(B, \chi)$ in the CwA for
$\hat\CC$, it is sufficient to define~$B$ and a subset
$\{\chi\}(\Gamma) \subseteq (\Phi\times B)(\Gamma)$ for any object $\Gamma$ of $\CC$.
The subsets define a monomorphism $\{\chi\} \mono X \times B$ that uniquely determines
$\chi \colon \Phi\times B \to \Omega$ by the universal property of the subobject classifier.

The dependent product $\Pi_X Y \in \mathrm{Ty}(\Phi)$ is defined for
$X\in \mathrm{Ty}(\Phi)$ and $Y\in\mathrm{Ty}(\Phi \ltimes X)$.
Suppose $X=(B_X, \chi_X)$ and $Y=(B_Y, \chi_Y)$.
Then, one can define $\Pi_X Y$ to be the pair $(B_X \parmap B_Y, \chi)$,
where the predicate $\chi$ is defined such that $\chi(p, f)$
is equivalent to $\chi_X(p, x)  \iff \chi_Y((p, x), f(x))$.
The implication from left to right states that the function~$f$ must map any~$x$ from
the argument to a result of the correct dependency. The implication from right to left
states that~$f$ is not defined for arguments that are not actually in the right dependent
type.

The identity type $\equiv_X$ in $\mathrm{Ty}(\Phi \ltimes X \ltimes \pi_X^* X)$ is defined
by the pair $(1, \chi)$, where $\chi$ is specified by:
\[
  ((p, x), y) \in \{\chi\}(\Gamma)
  \iff
  x = y
\]

\subsection{Yoneda Universe}

It remains to define the type for the Yoneda universe and the rest of
the structure identified in Secs.~\ref{sect:simple} and~\ref{sect:dep}.
We do this for representative cases.

We define $\Obj \in \mathrm{Ty}(1)$ as $(U, \top)$, where $O$ is the constant presheaf of
objects of~$\CC$ and $\top$ is the predicate that is always true.

For the Yoneda Universe, we define the type $\kw{El}\in \mathrm{Ty}(1 \ltimes \Obj)$
to be the pair $(M, \chi)$, where~$M$ is the presheaf with
$M(\Gamma) = \{ f \in \CC(\Gamma, \Delta) \mid \text{$\Delta$ an object of~$\CC$}\}$
and pre-composition as action and where
$\chi \colon (1\ltimes \ctx) \times M \to \Omega$
is defined by
\[
  ((*, \Delta), f) \in \{\chi\}(\Gamma)
  \iff
  f\in \CC(\Gamma, \Delta)
  \enspace.
\]
Compare this to the definition of the Yoneda embedding:
\[
  f \in \y(\Delta)(\Gamma)
  \iff
  f\in \CC(\Gamma, \Delta)
\]
The type~$\kw{El}$ is thus just the Yoneda embedding $\y(\Delta)$,
considered as a type depending on a variable $\Delta \colon \Obj$.

We next consider the structure from Sec.~\ref{sect:simple} in this interpretation.

\begin{lemma}
  When interpreted in the CwA for\/~$\hat\CC$,
  closed terms of type $\Obj$ correspond to
  to objects of $\CC$.
\end{lemma}
The lemma allows us to identify terms of type~$\Obj$ in the dependent type theory
for~$\hat\CC$ with objects in~$\CC$.

\begin{lemma}
  In the interal type theory of\/~$\hat\CC$, a term of type $\mpi x\of \Obj.\, X$
  corresponds to a family of terms $\bigl(t_A\colon X[A/x] \bigr)_A$, where~$A$ ranges
  over all objects of~$\CC$.
\end{lemma}
The point is that $\hat\CC$ does not impose a naturality condition on functions
out of $\Obj$.
It suffices to look at the function value at all possible arguments.

These two lemmas justify the terms $\kw{unit}$, $\kw{times}$ and $\kw{arrow}$
that represent the objects of~$\CC$ in $\hat\CC$.

We next look at the universe~$\CEl$ itself.
First we note that the interpretation of dependent types in a CwA is such that the
interpretation of closed types amounts to the standard interpretation of types in a
cartesian closed category. In particular, a closed type~$X$ corresponds to an object
of~$\CC$ and a function type $X\to Y$ between closed types~$X$ and~$Y$ is the exponential.
\begin{lemma}
  For closed $A \of \Obj$, the types $\El A$ and the object $\y(A)$ are isomorphic.
\end{lemma}
This can be seen by substituting~$A$ in the type $\CEl \in \mathrm{Ty}(1 \ltimes \Obj)$.

As a consequence, the denotation of closed terms of type $\El A \to \El B$
corresponds to morphisms $\y(A) \Rightarrow \y(B)$.
The interpretation of a term of type $\mpi a, b\of \Obj.\, \El a \to \El a$ is
just a family of such morphisms..

With this observation, Lemmas~\ref{lemma:terminal}--\ref{lemma:exponentials} correspond
to the standard preservation properties of the Yoneda embedding.
For example, that~$\y$ preserves exponentials can be seen because we have the following
natural isomorphism:
\begin{align*}
  (\y A\Rightarrow \y B) (\Gamma)
  &\ \iso\ \hat\CC(\y\Gamma, \y A \Rightarrow \y B)
    \ \iso\ \hat\CC(\y\Gamma \times \y A, \y B)
  \\
  &\ \iso\ \hat\CC(\y(\Gamma \times A), \y B)
   \ \iso\ \CC(\Gamma \times A, B)
  \\
  &\ \iso\ \CC(\Gamma, A \Rightarrow B)
   \ \iso\ \hat\CC(\y\Gamma, \y(A \Rightarrow B))
   \ \iso\ \y(A \Rightarrow B)(\Gamma)
\end{align*}
% TODO: move down

The box modality is interpreted using the $\flat$-comonad on~$\hat\CC$ from the main text.
Write $\varepsilon_X \colon \flat X \to X$ and $\nu_X \colon \flat X \to \flat\flat X$ for
its counit and comultiplication (the latter is actually the identity in our case).
We next describe the interpretation of the box modality~$[-]$.
It suffices to describe the action of~$[-]$ on projection maps (for types) and their sections
(for terms), since the CwA for~$\hat\CC$ is a splitting of the codomain fibration on~$\hat\CC$.
The type~$[X]$ is defined for any type~$X$ with a projection $\pi_X$ of the form $\pi_X\colon \flat \Gamma \ltimes X \to \flat \Gamma$.
It is defined as $\nu_X^*(\flat \pi_X)$.
A term $t\colon X$ corresponds to a section~$t\colon \flat \Gamma \to \{X\}$ of~$\pi_X$.
The term $[t]$ is interpreted by $\nu_X^* (\flat t)$.
Finally, for a term $s\colon [X]$, which is a section~$s$ of $\nu_X^*(\flat \pi_X)$,
we obtain a section of $\pi_X$ by post-composing~$s$ with the counit.
We use this to interpret the let-term for the box type.

The results in Sec.~\ref{sect:dep} are a direct internal formulation of the CwA-structure
of~$\CC$.
We consider Lemma~\ref{lem:depprod} as a representative example.
This lemma states an isomorphism between
$\mpi x\of \ElTm A \gamma.\, \ElTm B {(\kw{pair}\ \gamma\ x)}$
and $\ElTm {\Pi_AB} \gamma$.
To understand this, we first look at the interpretation of $\CElTm$. Suppose
$\Gamma \vdash A \type$ and
$\Gamma\comma x \of A  \vdash B \type$ in the CwA~$\CC$.
Write $\pi_A \colon \Gamma \ltimes A \to \Gamma$ and
$\pi_B \colon \Gamma \ltimes A \ltimes B \to \Gamma\ltimes A$
for their projection morphmisn.
The projection of the type $\gamma \of \El \Gamma \vdash \ElTm A \gamma$ is
then (up to isomorphism) given by $\y(\pi_A)$.
The projection of the type $\gamma \of \El {(\kw{cons}\ \Gamma\ A)} \vdash \ElTm B \gamma$ is
given by $\y(\pi_B)$.
The function~$\kw{pair}$ from Sec.~\ref{sect:dep} amounts to a morphism
$\kw{pair}\colon \y\Gamma \ltimes (\CElTm\ A) \to \y(\Gamma \ltimes A)$.
With this, we have the following isomorphism in slice categories.
\begin{align*}
  \CC/\Gamma (\id_{\Gamma}, \Pi_{y(\pi_A)} \kw{pair}^*\y(\pi_B))
  &\iso \CC/y(\Gamma \ltimes A) (\id_{\Gamma\ltimes A}, \y(\pi_B))
  \\
  &\iso \CC/(\Gamma \ltimes A) (\id, \pi_B)
    \iso \CC/\Gamma (\id_\Gamma, \pi_{\Pi_A B})
  \\
  &\iso \CC/\y\Gamma (\id_\Gamma, \y(\pi_{\Pi_A B}))
\end{align*}
This expresses the isomorphism between
$\mpi x\of \ElTm A \gamma.\, \ElTm B {(\kw{pair}\ \gamma\ x)}$
and $\ElTm {\Pi_AB} \gamma$.

\section{Interpretation of Simple Contextual Types}

To show soundness of the interpretation lemmas of simple contextual types from Sec.~\ref{sect:sctt},
we need substitution lemmas, of which we spell out representative cases here.

Substitution variables in context~$\Delta$ simply becomes substitution on the meta-level,
since the computation part is translated with a shallow embedding.
\begin{lemma} \leavevmode
  \begin{itemize}
  \item
    $
      \sem{\Delta\comma X\of U \comma \Delta' \semi \Phi  \vdash t \colon A}
      [\sem{\Delta\vdash C \colon U}/X] =
      \sem{\Delta\comma \Delta'[C/U] \semi \Phi  \vdash t[C/U] \colon A}
    $.
  \item
    $
      \sem{\Delta\comma X\of U \comma \Delta' \semi \Gamma  \vdash e \colon \tau}
      [\sem{\Delta\vdash C \colon U}/X] =
      \sem{\Delta\comma \Gamma[C/U] \semi \Phi  \vdash e[C/U] \colon \tau}
    $.
  \end{itemize}
\end{lemma}

Substitution on the $\Phi$-context becomes substitution for the new variable~$\gamma$,
which is essentially composition, as usual.
To define it, we need some notation.
We define a lifting from
$\sem{\Delta}\comma \gamma\of \El {\sem\Phi} \vdash t\colon \El{\sem{\Phi\comma x \of A}}$
to
$\sem{\Delta}\comma \gamma\of \El {\sem{\Phi\comma \Psi}} \vdash \textit{lift}_\Psi(t) \colon \El{\sem{\Phi\comma x \of A\comma \Psi}}$.
It is defined by
$\textit{lift}_{(\cdot)} (t) = t$ and
$\textit{lift}_{(\Psi,x\of C)} (t) = \lambda y.\, \kw{pair}\ (\textit{lift}_{\Psi}(t)[\kw{fst}\ \gamma/\gamma])\ (\kw{snd}\ \gamma)$.

\begin{lemma}
  $
  \sem{\Delta\semi \Phi\comma x\of A \comma \Psi \vdash t \colon B}[\textit{lift}_\Psi(\kw{pair}\ \gamma\ \sem{\Delta\semi \Phi\vdash s\colon A})/ \gamma] =
  \sem{\Delta\comma \Phi\comma \Psi \vdash t[s/x] \colon B}
  $.
\end{lemma}
Notice that in the interpretation of domain-level terms, a variable~$x$ from~$\Phi$ is
interpreted by projection from~$\gamma \colon \El {\sem\Phi}$.
In the main text, we have used projections, such as
$\pi_{(\Phi, x\of A), x} \colon \El {(\kw{times}\ \sem{\Phi}\ \sem{A})} \to \El \sem{A}$
for this purpose.
The lemma just states that pre-composing such a projection with a particular term
amounts to substituting the term.

The soundness lemma then follows using meta-level equations
and a substitution lemma.

\section{Interpretation of Contextual LF}

We follow Streicher's approach~\cite{streicher91} to the interpretation of the syntax
of dependent types by first defining the interpretation as a partial function by
induction on derivations.
The non-trivial cases are given in the main text and in the Agda code\footnotemark[1]\!.
To show that this interpretation is in fact total, we need weakening and substitution
lemmas.
We state these lemmas only for domain-level variables, as the other variables are again
moved to the meta level as in the simply-typed case.

\begin{lemma}[Weakening]
  \leavevmode
  \begin{itemize}
  \item
    $\kw{sub}\ \sem{\Delta\semi \Phi \vdash B\type}\ p =
    \sem{\Delta \semi \Phi\comma x \of A \vdash B\type}$
  \item
    $\kw{subElTm}\ (\sem{\Delta\semi \Phi \vdash t\colon B}[p\ \gamma/\gamma]) = \sem{\Delta \semi \Phi\comma x \of A \vdash t \colon B}$
  \end{itemize}
\end{lemma}
In the second part, recall that $\sem{\Delta\semi \Phi \vdash t\colon B}$ has type
$\ElTm {\sem{\Delta\semi \Phi \vdash B\type}} \gamma$, where~$\gamma$ is a variable of
type $\El \sem{\Phi}$. Thus, $\kw{subElTm}\ (\sem{\Delta\semi \Phi \vdash t\colon B}[p\ \gamma/\gamma])$
has type $\ElTm {(\kw{sub}\ \sem{\Delta\semi \Phi \vdash B\type}\ p)} \gamma$, which by
the first point has correct type for the right-hand side.
The proof of the lemma goes by induction on the derivation of $\sem{B}$ and $\sem{t}$.

\begin{lemma}[Substitution]
  \leavevmode
  \begin{itemize}
  \item
    $\kw{sub}\ \sem{\Delta\semi \Phi\comma x\of A \vdash B \type}\ (\lambda \gamma.\, \kw{pair}\ \gamma\ \sem{\Delta \semi \Phi \vdash s \colon A})
    = \sem{\Delta \semi \Phi \vdash B[s/x] \type}$
  \item
    $\kw{subElTm}\ (\sem{\Delta\semi \Phi\comma x \of A  \vdash t\colon B}[\kw{pair}\ \gamma\ \sem{\Delta \semi \Phi \vdash s \colon A}/\gamma])
    = \sem{\Delta \semi \Phi \vdash t[s/x] \colon B[s/x]}$
  \end{itemize}
\end{lemma}
The proof goes by showing a slightly stronger property (with a context $\Psi$ after the variable~$x\of A$)
by induction on the derivation of~$B$ and~$t$.

With the weakening and substitution lemmas, Lemma~\ref{lem:depint} follows by
induction on the showing that the partial interpretation is in fact total
by induction on derivations.

\section{Contextual LF}
\label{sect:contextuallf}

% TODO: $X$ sind jetzt Typen

We have spelled out the interpretation of simple contextual types to explain the essence
of our approach in a simple way.
Realistic systems with contextual types, such as Beluga, use
dependently-typed domain languages like \LF.

Dependent domain languages are useful to represent object-level languages more precisely.
In \LF, our running example of the untyped lambda-calculus can be refined into
an encoding of the simply-typed lambda calculus that allows only well-typed terms.
It is given by \LF type constants $\ty$ and $a \of\ty\vdash \kw{tm}\ a$ for
object-level types and terms.
Concrete object-level types are represented by a constant $\kw{o}\colon \ty$ for a base
type and a constant $\kw{arr} \colon \ty\to \ty\to \ty$ for function types.
Object-level terms are encoded using the constants
$\kw{app} \colon \Pi a,b\of \ty.\ \kw{tm}\ (\kw{arr}\ a\ b) \to \kw{tm}\ a \to \kw{tm}\ b$
and
$\kw{lam} \colon \Pi a,b\of \ty.\ (\kw{tm}\ a \to \kw{tm}\ b) \to  \kw{tm}\ (\kw{arr}\ a\ b)$.
The type dependencies are chosen so that one can only represent well-typed terms.

In the rest of this paper, we extend our semantical analysis to cover contextual types
over~\LF.
We consider the type system Contextual \LF, which is obtained from the simple contextual
type system by replacing the simply-typed domain language with~\LF.
The typing rules of Contextual LF in Fig.~\ref{fig:cttlf} are a direct generalisation of
the rules in Fig.~\ref{fig:cttstl}.
\begin{figure*}[t]
  \small
  \fbox{$\Delta\semi \Phi \vdash A \type$} : well-formed LF type
\[
  \begin{prooftree}[center=false]
    \Hypo{
      \Delta\vdash \Phi \colon \ctx
    }
    \Infer1{
      \Delta\semi \Phi \vdash \ty \type
    }
  \end{prooftree}
  \qquad
  \begin{prooftree}[center=false]
    \Hypo{
      \Delta\semi \Phi \vdash t \colon \ty
    }
    \Infer1{
      \Delta\semi \Phi \vdash (\tm\ t) \type
    }
  \end{prooftree}
  \qquad
  \begin{prooftree}[center=false]
    \Hypo{
      \Delta\semi \Phi\comma x \of A \vdash B \type
    }
    \Infer1{
      \Delta\semi \Phi \vdash \Pi x\of A.\, B \type
    }
  \end{prooftree}
\]

\fbox{$\Delta\semi \Phi \vdash t \colon A$} : for LF terms
\[
  \begin{prooftree}[center=false]
    \Hypo{\Delta \vdash \Phi \colon \ctx}
    \Hypo{\Delta \semi \Phi \vdash A \type}
    \Infer2{
      \Delta\semi \Phi\comma x\of A \vdash x \colon A
    }
  \end{prooftree}
  \quad
  \begin{prooftree}[center=false]
    \Hypo{\Delta \vdash \Phi \colon t \colon B}
    \Hypo{\Delta \semi \Phi \vdash A \type}
    \Infer2{
      \Delta\semi \Phi\comma x\of A \vdash t \colon B
    }
  \end{prooftree}
\quad
  \begin{prooftree}[center=false]
    \Hypo{
      \Delta\semi \Phi\comma x\of A \vdash t \colon B
    }
    \Infer1{
      \Delta\semi \Phi \vdash \lambda x \of A.\, t \colon \Pi x\of A.\, B
    }
  \end{prooftree}
\]
\[
  \begin{prooftree}[center=false]
    \Hypo{
      \Delta\semi \Phi \vdash s \colon \Pi x \of A.\, B
    }
    \Hypo{
      \Delta\semi \Phi \vdash t \colon A
    }
    \Infer2{
      \Delta\semi \Phi \vdash s\ t \colon B[t/x]
    }
  \end{prooftree}
  \quad
  \begin{prooftree}[center=false]
    \Hypo{
      \Delta \vdash C \colon (\CT \Phi A)
    }
    \Hypo{
      \Delta\semi \Psi \vdash \sigma \colon \Phi
    }
    \Infer2{
      \Delta\semi \Psi \vdash \esub C \sigma \colon A[\sigma/\Phi]
    }
  \end{prooftree}
  \qquad
  \begin{prooftree}[center=false]
    \Hypo{
      \Delta \vdash \Phi\colon \ctx
    }
    \Infer1{
      \Delta\semi \Phi \vdash c \colon A
    }
  \end{prooftree}
\]
where $c\colon A$ is one of the constants $\kw{o}$, $\kw{arr}$, $\kw{app}$ and $\kw{lam}$,
as described in the text.

\fbox{$\Delta\semi \Phi \vdash \sigma \colon \Psi$} : domain-level substitutions
\[
  \begin{prooftree}[center=false]
    \Hypo{
      \Delta \vdash \Phi \colon \ctx
    }
    \Infer1{
      \Delta\semi \Phi \vdash \cdot \colon \cdot
    }
  \end{prooftree}
  \qquad
  \begin{prooftree}[center=false]
    \Hypo{
      \Delta \vdash \Phi\comma \overline{x\of A} \colon \ctx
    }
    \Infer1{
      \Delta\semi \Phi\comma \overline{x\of A} \vdash \id_\Phi \colon \Phi
    }
  \end{prooftree}
  \qquad
  \begin{prooftree}[center=false]
    \Hypo{
      \Delta\semi \Phi \vdash \sigma \colon \Psi
    }
    \Hypo{
      \Delta \semi \Psi \vdash A \type
    }
    \Hypo{
      \Delta\semi \Phi \vdash t \colon A[\sigma/\Psi]
    }
    \Infer3{
      \Delta\semi \Phi \vdash (\sigma, t) \colon (\Psi\comma x\of A)
    }
  \end{prooftree}
\]

\fbox{$\Delta\vdash C \colon U$} : contextual objects
\[
  \begin{prooftree}[center=false]
    \Hypo{
      \vdash \Delta \context
    }
    \Hypo{
      \Delta(X) = U
    }
    \Infer2{
      \Delta \vdash X \colon U
    }
  \end{prooftree}
  \quad
  \begin{prooftree}[center=false]
    \Hypo{
      \Delta\semi \Phi \vdash t \colon A
    }
    \Infer1{
      \Delta \vdash (\CT \Phi t) \colon (\CT \Phi A)
    }
  \end{prooftree}
  \quad
  \begin{prooftree}[center=false]
    \Hypo{
      \vdash \Delta \context
    }
    \Infer1{
      \Delta \vdash \cdot \colon \ctx
    }
  \end{prooftree}
  \quad
  \begin{prooftree}[center=false]
    \Hypo{
      \Delta \vdash \Phi \colon \ctx
    }
    \Hypo{
      \Delta \semi \Phi \colon A \type
    }
    \Infer2{
      \Delta \vdash \Phi\comma x\of A \colon \ctx
    }
  \end{prooftree}
\]

We omit the rules for
{$\Delta\vdash \theta \colon \Delta'$}
and
{$\Delta\semi \Gamma \vdash e \colon \tau$},
which are as in  Fig.~\ref{fig:cttstl},
as well as  the straightforward well-formedness rules for {$\vdash \Delta \context$}, {$\Delta \vdash \tau \comptype$} and
{$\Delta\vdash U \ctxtype $}.
\caption{Typing Rules of Contextual LF}
\label{fig:cttlf}
\end{figure*}

\section{Categories with Attributes}
\label{sect:cattributes}

To define a semantics for Contextual \LF, we need to model dependent types.  There are a
number of essentially-equivalent notions of models of dependent type theory, such as
Categories with Families~\cite{Dybjer:TYPES95}, Categories with
Attributes~\cite{Cartmell:JAL86}, Comprehension
Categories~\cite{Jacobs:TCS93}, etc.
For our purposes, \emph{Category with Attributes} (CwA) in the formulation of~\cite{Hofmann:NI97} are convenient.

\begin{definition}
  \label{def:cwa}
A \emph{category with attributes} given by the following data.
\begin{itemize}
\item A category $\CCtx$, called \emph{category of contexts}, with a terminal object.

\item
  A functor $\mathrm{Ty} \colon \op{\CCtx} \to \mathrm{Set}$.

\item For each type $X\in \mathrm{Ty}(\Phi)$, an object $\Phi \ltimes X$
  and a morphism $\pi_X \colon \Phi \ltimes X \to \Phi$ in $\CCtx$.
  We call $\pi_X$ a \emph{projection morphism}.

\item
  For all $\sigma \colon \Psi \to \Phi$ in $\CCtx$ and $X\in \mathrm{Ty}(\Phi)$,
  a morphism $q(\sigma,X)$  making the following diagram in~$\CCtx$ a pullback.
  \quad
    \xymatrix@C=2cm@R=0.7cm{
      \Psi \ltimes \mathrm{Ty}(\sigma)(X)
      \ar[r]^-{q(\sigma, X)}
      \ar[d]_{\pi_{\mathrm{Ty}(\sigma)(X)}}
      \pullbackcorner[ul]
      &
       \Phi \ltimes X
      \ar[d]^{\pi_X}
      \\
      \Psi
      \ar[r]_{\sigma}
      &
      \Phi
    }
\end{itemize}
\end{definition}
The category~$\CCtx$ represents contexts and substitutions.
Its objects represent contexts. The terminal object is the empty context.
A morphism $\sigma \colon \Phi \to \Psi$ in $\CCtx$ represents a substitution that defines
a term in context~$\Phi$ for each variable in~$\Psi$.

The functor $\mathrm{Ty}$ represents dependent types and type substitution.
For an object~$\Phi$ of $\CCtx$, the set~$\mathrm{Ty}(\Phi)$ is the set of types
in context~$\Phi$.
For any morphism $\sigma \colon \Psi \to \Phi$, the function
$\mathrm{Ty}(\sigma) \colon \mathrm{Ty}(\Phi) \to \mathrm{Ty}(\Psi)$ explains how to
apply the substitution~$\sigma$ to the types in context~$\Phi$.
%
% The result is a type in context~$\Psi$. % komisch

The object $\Phi \ltimes X$ represents the context ``$\Phi \comma x\of X$''.
The projection $\pi_X$ is the weakening substitution. For example, if we have
a type $Y\in\mathrm{Ty}(\Phi)$, then $\mathrm{Ty}(\pi_X)(Y) \in \mathrm{Ty}(\Phi\ltimes X)$
should be understood as the same type~$Y$ after weakening with a variable of type~$X$.

The morphism $q(\sigma, X)$ lifts the substitution~$\sigma$ to an extended context.
It corresponds to a substitution of the form $(\sigma,x)$ in the type theories
of Secs.~\ref{sect:sctt} and~\ref{sect:contextuallf}. % TODO: ist das klarer als vorher?

The definition of a CwA does not mention terms, since these are considered a derived
concept.
A term of type $X\in\mathrm{Ty}(\Phi)$ in context~$\Phi$ can be identified with a
\emph{section of $\pi_X$}, which is a morphism $\sigma \colon \Phi \to \Phi \ltimes X$
with the property $\pi_X \circ \sigma = \id$.
%
% ((Warum wird das überhaupt gesagt?))
% If one represents the terms of type~$X$ by the set of all sections of~$\pi_X$, then one
% obtains a Category with Families, see~\cite{Hofmann:LICS99} for details.

Having defined CwAs, we can say a few words about the type theory for~$\hat\CC$ that we
have described in Sec.~\ref{sect:simple}.
% TODO: klarer machen:
One can define a CwA with~$\hat\CC$ as the category of contexts.
Let us spell out the projections of a few types.
The type $\Obj \in \mathrm{Ty}(1)$ has the projection $\pi_\Obj \colon O \to 1$, where $O(\Gamma)$ is the set of objects of~$\CC$.
The type $\CEl \in \mathrm{Ty}(O)$ has the projection $\pi_\CEl\colon M \to O$, where $M(\Gamma)$ is the set of pairs $(\Delta, f)$
with $\Delta \in O(\Gamma)$ and $f\in \CC(\Gamma, \Delta)$,
and where $\pi_\CEl(\Delta, f) = \Delta$.
Note that any object~$A$ of~$\CC$ defines a map $A\colon 1 \to O$, which corresponds to a term of type $\Obj$.
Substituting the type $\CEl$ with this map, gives us a type whose projection is (up to isomorphism)
the pullback of~$\pi_\CEl$ along~$A$.
This is easily seen to be just $\y A \to 1$, which justifies our view of~$\CEl$ as a syntax for the Yoneda embedding.

\section{Presheaves on a Small Category with Attributes}
\label{sect:dep}

With the notion of CwA, we can now come to modelling Contextual \LF.
We still use a presheaf category~$\hat\CC$ as before,
but we now use a CwA~$\CC$ instead of a cartesian closed category.
Thus, assume from now on that~$\CC$ is a CwA, e.g.~the term model of~\LF.
We now again consider the Yoneda embedding of the CwA~$\CC$ into~$\hat\CC$ in type-theoretic
terms, as in Sec.~\ref{sect:simple}.

\subsection{Yoneda CwA}

% TODO: this used to be Obj
We write $\Ctx$ for the type of all the objects of $\CC$.
In the canonical model, these would be LF contexts.
The type $\Ty c$ is the set of types in context~$c$, as defined as part of the CwA.
\begin{align*}
  &\vdash \Ctx\type
  &
  &c\of \Ctx \vdash \Ty c\type
\end{align*}
Both $\Ctx$ and $\Ty c$ have trivial presheaf structure, i.e.~$[\Ctx]=\Ctx$ and $[\Ty c]=\Ty c$.

Because of the dependency structure of dependently typed contexts, we cannot simply model them anymore using products as we did in Sec \ref{sect:sctt}. Instead, contexts are represented using the constants $\kw{nil}$ and $\kw{cons}$:
\begin{align*}
  &\vdash \kw{nil} \colon \Ctx
  &
  &\vdash \kw{cons} \colon \mpi c\of \Ctx.\, \mpi a\of (\Ty c).\, \Ctx
\end{align*}
The constant~$\kw{nil}$ denotes the terminal object
and $\kw{cons}\ c\ a$ stands for $c \ltimes a$
in the CwA~$\CC$.
%
%We write $\kw{nil}$ instead of $\kw{unit}$ as before, since contexts are intended to be read
%as lists.
% NEEDED SPACE (and it's said already above the maths display)

As before, we consider the contexts as codes of a universe $\CEl$.
\[
  c\of \Ctx \vdash \El c\type
\]
The type $\El c$ has the same definition as above and is essentially just the Yoneda
embedding.
It thus represents all global elements of the context $c$ in~$\CC$, i.e.~all substitutions
with codomain~$c$.
One should therefore think of a term of type~$\El c$ as a tuple of domain-level terms, one
for each declaration in the context represented by~$c$.
A function $\El c \to \El d$ corresponds to a context morphism $c\to d$ in~$\CC$,
as the Yoneda embedding is full and faithful.

The CwA-structure of $\CC$ now induces the following terms in $\hat\CC$.
\begin{align*}
  & \vdash \kw{terminal} \colon \El \kw{nil} % SPACE: das koennte man nach rechts schieben
  \\
  c\of \Ctx\comma a \of (\Ty c)
  &\vdash p \colon \El\ {(\kw{cons}\ c\ a)} \to \El c
  \\
  c,d\of \Ctx
  &\vdash \kw{sub} \colon \mpi a\of(\Ty d).\, \mpi f\of (\El c \to \El d).\, \Ty c
  \\
  c,d\of \Ctx
  &\vdash q \colon \mpi a\of(\Ty d).\, \mpi f\of (\El c \to \El d).\,
    \El {(\kw{cons}\ c\ (\kw{sub}\ a\ f))} \to \El {(\kw{cons}\ d\ a)}
\end{align*}

The following lemmas correspond to the CwA-axioms.
\begin{lemma}
  Substitution is functorial:
  We have $\kw{sub}\ a\ (\lambda x.x) = a$ and
  $\kw{sub}\ a\ (g\circ f) = \kw{sub}\ (\kw{sub}\ a\ g)\ f$
  for all $c \of \Ctx$, $a \of (\Ty c)$,
  $f\of \El e \to \El d$ and $g\of \El d \to \El c$.
\end{lemma}

\begin{lemma}
  The type $\El {\kw{nil}}$ is terminal, which means that any $x\of \El {\kw{nil}}$
  satisfies $x = \kw{terminal}$.
\end{lemma}

The pullback property from Def.~\ref{def:cwa} is stated internally as follows:
\begin{lemma}
  Let $c,d \of \Ctx$, $a \of (\Ty c)$ and $f\colon \El d \to \El c$.
  Then we have $ p\ (q\ a\ f\ \gamma) = f\ (p\ \gamma)$ for all $\gamma \of \El c$.
  Moreover, for all $x\of \El {(\kw{cons}\ d\ a)}$ and $\gamma \of \El c$,
  there exists a unique $y\of \El {(\kw{cons}\ c\ (\kw{sub}\ a\ f))}$
  with $p\ y = \gamma$ and $q\ a\ f\ y = x$.
  % \[
  %   \xymatrix@C=1.5cm{
  %      \El {(\kw{cons}\ c\ (\kw{sub}\ a\ f))}
  %     \ar[r]^-{q\ a\ f}
  %     \ar[d]_{p}
  %     \pullbackcorner[ul]
  %     &
  %     \El {(\kw{cons}\ d\ a)}
  %     \ar[d]^{p}
  %     \\
  %     \El c
  %     \ar[r]_{f}
  %     &
  %     \El d
  %   }
  % \]
  % This means the square commutes, i.e.\ $ p\ (q\ a\ f\ \gamma) = f\ (p\ \gamma)$ for all $\gamma \of \El c$, and,
  % for all $x\of \El {(\kw{cons}\ d\ a)}$ and $\gamma \of \El c$,
  % there exists $y\of \El {(\kw{cons}\ c\ (\kw{sub}\ a\ f))}$
  % with $p\ y = \gamma$ and $q\ a\ f\ y = x$,
  % and any other~$y'$ with this property is equal to~$y$.
\end{lemma}

For working with the CwA structure, it is useful to define a dependent type
\begin{align*}
  c\of \Ctx \comma
  a \of (\Ty c) \comma
  \gamma \of (\El c)
  &\vdash
    \ElTm a \gamma \type
  % \\
  % c\of \Ctx \comma
  % a \of (\Ty c) \comma
  % \gamma \of (\El c)
  % &\vdash
  % \ElTm a \gamma\ :=\ \Sigma v\of \El{(\kw{cons}\ c\ a)}.\, (p\ v) = \gamma
\end{align*}
by $\ElTm a \gamma\ :=\ \Sigma v\of \El{(\kw{cons}\ c\ a)}.\, (p\ v) = \gamma$.
This $\Sigma$-type consists of all pairs~$<v, w>$ where~$v$
has type $\El{(\kw{cons}\ c\ a)}$ and where~$w$ is a proof of $(p\ v) = \gamma$.
%
%For $t\colon \ElTm a \gamma$, we write $\{t\} \colon \El{(\kw{cons}\ c\ a)}$
%for its first component.

The type $\ElTm a \gamma$ thus consists of all values in $\El {(\kw{cons}\ c\ a)}$ whose first projection is~$\gamma$.
If one considers $\gamma \of \El c$ as a tuple of domain-level terms (one term for each
variable in the context represented by $c$), then $\ElTm a \gamma$ represents all the
terms that can be appended to this tuple to make it into one of type $\El {(\kw{cons}\ c\ a)}$.
Accordingly, we can define a pairing operation and a second projection
\begin{align*}
  c\of \Ctx\comma a\of (\Ty c)
  &\vdash
    \kw{pair} \colon \mpi \gamma \of (\El c).\, \ElTm a \gamma \to \El {(\kw{cons}\ c\ a)}
  \\
  c\of \Ctx\comma a\of (\Ty c)
  &\vdash
  p' \colon \mpi \gamma \of \El {(\kw{cons}\ c\ a)}.\, \ElTm a {(p\ \gamma)}
\end{align*}
by $\kw{pair} := \lambda \gamma.\, \lambda <v, p>.\, v$ and
$p':=\lambda \gamma.\, <\gamma, \mathrm{refl}>$.
The first projection~$p$ was already defined.

The next lemma relates $\CElTm$ to substitution.
Its proof uses Lemma~\ref{lem:pullback}.
\begin{lemma}
  \label{lem:pullback}
  For $c, d\colon \Ctx$, $a\colon (\Ty c)$, $f\colon \El d \to \El c$ and
  $\gamma \colon (\El d)$, there is an isomorphism
  $\kw{subElTm} \colon \ElTm{a}{(f\ \gamma)} \to \ElTm{(\kw{sub}\ a\ f)}{\gamma}$.
  We write $\kw{subElTm}^{-1}$ for its inverse.
\end{lemma}

Finally, we can define a type of domain-level terms
by $\Tm c a := \mpi \gamma \of (\El c).\, \ElTm a \gamma$.
This type represents domain-level terms just as $\Ty c$ represents domain-level types.
It is not hard to show that $\Tm c a$ is isomorphic to the type of sections of
$p\colon \El{(\kw{cons}\ c\ a)} \to \El c$, cf.~Sec.~\ref{sect:cattributes}.
We prefer to use $\CElTm$ over~$\CTm$, since it allows us to move domain-level
abstractions into meta-level abstractions, e.g.~in Lemma~\ref{lem:depprod} below.

So far, we have only exposed the CwA structure of~$\CC$ in~$\hat\CC$.
Dependent products in the domain language are lifted to $\hat\CC$ by the following
lemma, which generalises Lemma~\ref{lemma:exponentials}.
\begin{lemma}
  \label{lem:depprod}
  If the CwA~$\CC$ has dependent products, then the internal type theory of\/~$\hat\CC$
  has the following terms, in which~$\Gamma$ abbreviates
  $c \of \Ctx\comma
  a \of (\Ty c) \comma
  b \of (\Ty {(\kw{cons}\ c\ a)}) \comma
  \gamma \of \El c$.
  \begin{align*}
    c \of \Ctx
    &\vdash \Pi \colon \forall a\of (\Ty c).\, \Ty {(\kw{cons}\ c\ a)} \to \Ty c
    \\
    \Gamma
    &\vdash
      \kw{\ensuremath{\Pi}-e}\colon
      \ElTm {(\Pi\ a\ b)} \gamma
      \to \mpi x\of (\ElTm a \gamma).\ \ElTm b (\kw{pair}\ \gamma\ x)
    \\
    \Gamma
    &\vdash
      \kw{\ensuremath{\Pi}-i}\colon
      (\mpi x\of (\ElTm a \gamma).\ \ElTm b (\kw{pair}\ \gamma\ x))
      \to
      \ElTm {(\Pi\ a\ b)} \gamma
  \end{align*}
  Moreover, $\kw{\ensuremath{\Pi}-i}$ and $\kw{\ensuremath{\Pi}-e}$ are mutually inverse.
\end{lemma}
The term $(\Pi\ a\ b)$ in the type theory for $\hat\CC$ represents the dependent product
type in~$\CC$.
It is well-behaved with respect to substitution. % TODO: say more, e.g. (Beck-Chevalley)?

Object-level term constants in the type theory modelled by~$\CC$, such as $\ty$, $\kw{tm}$,
$\kw{app}$ and $\kw{lam}$ from above can be lifted using~$\CElTm$.
We use the same name for the lifted constants.
\begin{align*}
  c\of \Ctx
  &\vdash \ty \colon \Ty c
  &
  \Gamma &\vdash \kw{o} \colon \ElTm {\ty} \gamma
  \\
  c\of \Ctx &\vdash \kw{tm} \colon \Ty {(\kw{cons}\ c\ \ty)}
  &
  \Gamma
  &\vdash \kw{arr} \colon \ElTm {\ty} \gamma \to \ElTm {\ty} \gamma \to \ElTm {\ty} \gamma
  \\
  \Delta
  &\vdash \rlap{$\kw{app} \colon
    \ElTm {\kw{tm}} {(\kw{pair}\ \gamma\ (\kw{arr}\ a\ b))} \to
    \ElTm {\kw{tm}} {(\kw{pair}\ \gamma\ a)} \to
    \ElTm {\kw{tm}} {(\kw{pair}\ \gamma\ b)}$}
 \\
  &\vdash \rlap{$\kw{lam} \colon
    \left(\ElTm {\kw{tm}} {(\kw{pair}\ \gamma\ a)} \to \ElTm {\kw{tm}} {(\kw{pair}\ \gamma\ b)} \right) \to
    \ElTm {\kw{tm}} {(\kw{pair}\  \gamma\ (\kw{arr}\ a\ b))}$}
\end{align*}
where~$\Gamma$ abbreviates $c\of \Ctx\comma \gamma\of (\El c)$ and~$\Delta$ abbreviates
$\Gamma\comma a, b \of (\ElTm{\ty} \gamma)$.
Notice how~$\kw{lam}$ uses higher-order abstract syntax at the meta level.
For this, it seems to be essential to use $\CElTm$ rather than a formulation with~$\CTm$.
% TODO: Say something about substitution equations?

\section{Interpreting Contextual LF}

Having outlined the structure of presheaves over a CwA, we now use this
structure to model Contextual~\LF in~$\hat\CC$.
We assume that $\CC$ is a model of \LF, i.e.~a CwA with dependent products, and that it
models the constants for $\ty$ and $\kw{tm}$ from the preceding section.
The term model is a canonical example for~$\CC$.

With type dependencies, we cannot define the interpretation of types and terms separately,
but must define the whole interpretation by induction on the derivation.
As before, we denote derivations simply by their conclusion or the principal part thereof.
With this understanding, we can define the interpretation of contextual types
($\Delta\vdash U \ctxtype$) and computation types
($\Delta \vdash \tau \comptype$) almost exactly as before.
\begin{align*}
    \sem{\ctx} &= \mathtt{Ctx}
  &
    \sem{[U]} &= \sem{U}
  \\
    \sem{\CT \Phi A} &= [\forall \gamma \of \El{\sem{\Phi}}.\, \ElTm{\sem{A}}\gamma]
  &
    \sem{\tau_1 \to \tau_2} &= \sem{\tau_1} \to \sem{\tau_2}
  \\
               &
  &
    \sem{\mpi X \of U\dt \tau} &= \mpi X \of \sem{U}\dt \sem{\tau}
\end{align*}
This definition makes reference to the interpretation of contextual objects
(via $\Delta \vdash \Phi\colon \ctx$) and to LF types (via $\Delta\semi \Phi \vdash A \type$).
Before we outline the interpretation of such judgements, it is useful to
formulate the typing invariants of the interpretation.

\begin{lemma}
  \label{lem:depint}
  The interpretation maintains the following invariants:
  \begin{itemize}
  \item
    If $\Delta \semi \Phi \vdash A \type$, then
    $\sem{\Delta} \vdash \sem{A} \colon \Ty{\sem{\Phi}}$.
  \item If $\Delta\semi \Phi \vdash t \colon A$ then
    $\sem{\Delta} \comma \gamma\of \El\sem{\Phi} \vdash \sem{t} \colon \ElTm {\sem{A}} \gamma$.
  \item
    If $\Delta\semi \Phi \vdash \sigma \colon \Psi$ then $\sem{\Delta}\comma \gamma\of \El\sem{\Phi} \vdash \sem{\sigma} \colon \El\sem{\Psi}$.
  \item
    If $\Delta \vdash U \ctxtype$ then $\sem{\Delta} \vdash \sem{U} \type$.
  \item
    If $\Delta \vdash C \colon U$ then $\sem{\Delta} \vdash \sem{C} \colon \sem{U}$.
  \item
    If $\Delta \vdash \theta \colon \Delta'$ then $\sem{\Delta} \vdash \sem{\theta} \colon \sem{\Delta'}$.
  \item
    If $\Delta \vdash \tau \comptype$ then $\sem{\Delta} \vdash \sem{\tau} \type$.
  \item
    If $\Delta\semi \Gamma \vdash e \colon \tau$ then $\sem{\Delta}\comma \sem{\Gamma} \vdash \sem{e} \colon \sem{\tau}$.
  \end{itemize}
\end{lemma}
With these invariants in mind, the interpretation is essentially straigthforward.
For example, \LF types and contextual objects are interpreted by:
\begin{align*}
  \sem{\Delta \semi \Phi \vdash \kw{ty} \type} &= \kw{ty}
  \\
  \sem{\Delta \semi \Phi \vdash \kw{tm}\ t \type} &= \kw{sub}\ \kw{tm}\ (\lambda \gamma.\, \sem{\Delta \semi \Phi \vdash t \of \kw{ty}})
  \\
  \sem{\Delta \semi \Phi \vdash \Pi x\of A.\, B \type} &= \Pi\ \sem{ \Phi \vdash A \type}\ \sem{\Delta \semi \Phi\comma x \of A \vdash B \type }
  \\
  \sem{\Delta\semi \Phi\comma x\of A \vdash x \colon A} &= \kw{subElTm} (p'\ \gamma) \text{ (variable rule)}
  \\
  \sem{\Delta\semi \Phi\comma x\of A \vdash t \colon A} &= \kw{subElTm}\ \sem{\Delta\semi \Phi \vdash t \colon A}[p\ \gamma / \gamma]
                                                          \text{ (weakening rule)}
  \\
  \sem{\lambda x \of A.\, t} & = \kw{$\Pi$-i}\ (\lambda x\of \sem{A}.\, \sem{t}[\kw{pair}\ \gamma\ x/ \gamma])
  \\
  \sem{s\ t} & = \kw{subElTm}\ (\kw{$\Pi$-e}\ \sem{s}\ \sem{t})
  \\
  \sem{\esub C \sigma} & = \tlet {[X]} {\sem{C}} {[\lambda \gamma \of\sem{\Psi}.\, \kw{subElTm}\ (X\ \sem{\sigma}) ]}
\end{align*}
The definition of~$\pi$ from Sec.~\ref{sect:stlint} is now built into the explicit weakening rule.
The term $\kw{subElTm}$ is used for type substitution.
In the interpretation of application, for example, $(\kw{$\Pi$-e}\ \sem{s}\ \sem{t})$ has
type $\ElTm{\sem{B}}{(\kw{pair}\ \gamma\ \sem{s})}$.
By using $\kw{subElTm}$, we get a term of type
$\ElTm{(\kw{sub}\ \sem{B}\ (\lambda \gamma.\, \kw{pair}\ \gamma\ \sem{s}))}{\gamma}$, which is equal to
the required $\ElTm{\sem{B[s/x]}}{\gamma}$ (making use of extensional equality in the meta-theory).

Due to the type dependencies, the definition of the interpretation needs some care.
In the example of application, we have used that
$(\kw{sub}\ \sem{B}\ (\lambda \gamma.\, (\kw{pair}\ \gamma\ \sem{s})))$ and $\sem{B[s/x]}$ are
equal, but this information is not available during the definition of $\sem{-}$.
The standard approach, due to Streicher~\cite{streicher91}, is to consider
the definition of~$\sem{-}$ a priori as a partial function that is undefined if types do not match.
Then one proves weakening and substitution lemmas using the partial definition of~$\sem{-}$.
With these lemmas, one can then show by induction on derivations that~$\sem{-}$ is
in fact total after all.
We elide such details in this paper.

%%% Local Variables:
%%% TeX-master: "fscd"
%%% End:
